# Supplementary material for: Securing Wi-Fi 6 Connection Establishment Against Relay and Spoofing Threats
Source: arXiv:2501.01517 source file (2025-01-02)
Supplement: Supplementary file 1 [file 10.appendix.tex]

\section*{Appendix}

%\subsection{Important Notations}\label{notation-section}

mjyfjhlkj

%\subsection{Detailed Model for Model Checking}\label{detailed-model}

\begin{figure*}[h]
    \centering
    \includegraphics[scale=0.3]{figures/mc_solution.png}
    \caption{Detailed version of the connection establishment system model with our proposed solution in place ($\mathcal{M} $)}.\label{fsms}
   % \vspace{-0.35in}
\end{figure*}
